# Supplementary material for: Kinematic dependence of azimuthal anisotropies in $p$$+$Au, $d$$+$Au, $^3$He+Au at $\sqrt{s_{_{NN}}}$ = 200 GeV
Source: arXiv:2107.06634 ancillary file (2022-02-03)
Supplement: Supplementary file 1 [file supp_mat.pdf]

# The full set of $\Delta\phi$ correlations coefficients

The two-particle correlations themselves contain valuable information – the details of which may be of high interest only to some readers. Therefore, we include in this supplemental material a subset of the two-particle correlations after event-mixing correction from the combinations BBCS-FVTXS (Fig. 13), BBCS-FVTXN (Fig. 14), FVTXS-FVTXN (Fig. 15), CNT-BBCS (Fig. 16), CNT-FVTXS (Fig. 17), and CNT-FVTXN (Fig. 18). The correlations shown involving the CNT are for tracks with $0.2 < p_T < 3.0$ GeV/$c$. The panels include results from minimum-bias (MB) $p$+$p$ collisions, 0%–5% central $p$+Au, $d$+Au, and $^3$He+Au collisions. We note that the $p$+$p$ collisions are triggered on the requirement of at least one hit in the BBCS and one hit in the BBCN and thus selected approximately 55% ± 5% of the 42 mb inelastic cross section—for details on the trigger and potential bias see Ref. [34].

Tables V–XX show the numbers for the full set of correlations coefficients. For this larger set we include only the extracted Fourier coefficients $c_1, c_2, c_3, c_4$ and their statistical uncertainties. For $p_T$-integrated coefficients, those with the CNT are for tracks with $0.2 < p_T < 3.0$ GeV/$c$. Because only the CNT has tracks with $p_T$ information, combinations including the CNT will have a large number of such correlations. Four sets of four tables each are shown for $p$+$p$ (Tables V–VIII), $p$+Au (Tables IX–XII), $d$+Au (Tables XIII–XVI), and $^3$He+Au (Tables XVII–XX) collisions. For each collision system the four tables show first the $p_T$-integrated coefficients, then the $p_T$-dependent coefficients for the CNT-BCS, CNT-FVTXS, and CNT-FVTXN correlations, respectively.

We highlight that the CNT track sample includes strict quality cuts and that systematic uncertainties from background contributions are highly subdominant. In contrast, the FVTX track sample requires hits in only 3 of 4 layers and has no momentum information available. In addition, the performance in terms of acceptance, efficiency, and background in the FVTX can vary from year to year, particularly during the earlier commissioning phase. As mentioned in the main text, the BBC simply sums charge deposits and has substantial contributions, of order 50%, from particles scattering in from outside the nominal $3.1 < |\eta| < 3.9$ acceptance. Thus, the $c_n$ coefficients from the FVTX and BBC should not be viewed strictly as physics quantities. In the case of $p$+$p$ collisions, there are differences between the CNT-FVTXS and CNT-FVTXN extracted coefficients despite the symmetric collision system. Thus, for example, the 20% difference in the $c_2$ coefficients is an indication of these detector specific contributions. Accounting for these effects in interpreting the coefficients and using them between systems for nonflow corrections requires appropriate caveats.

[34] A. Adare, *et al.* (PHENIX Collaboration) "Centrality categorization for $R_{p(d)+A}$ in high-energy collisions," Phys. Rev. C, **90**, 034902 (2014).

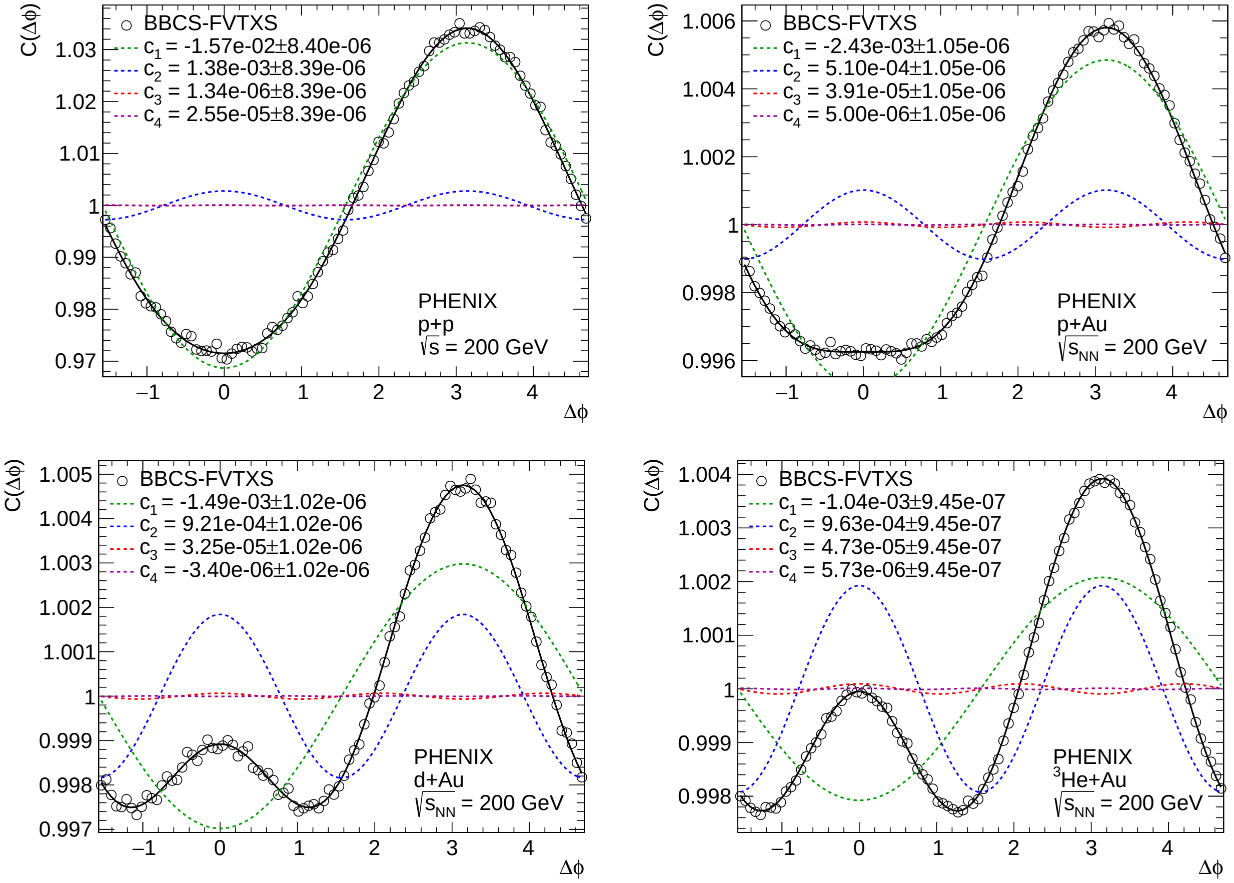


FIG. 13. BBCS-FVTXS $\Delta\phi$ distribution in MB $p$+$p$ and 0%–5% central $p$+Au, $d$+Au, and $^{3}$He+Au. The measured correlation function is shown with open black circles and the fit is shown as a solid black line.

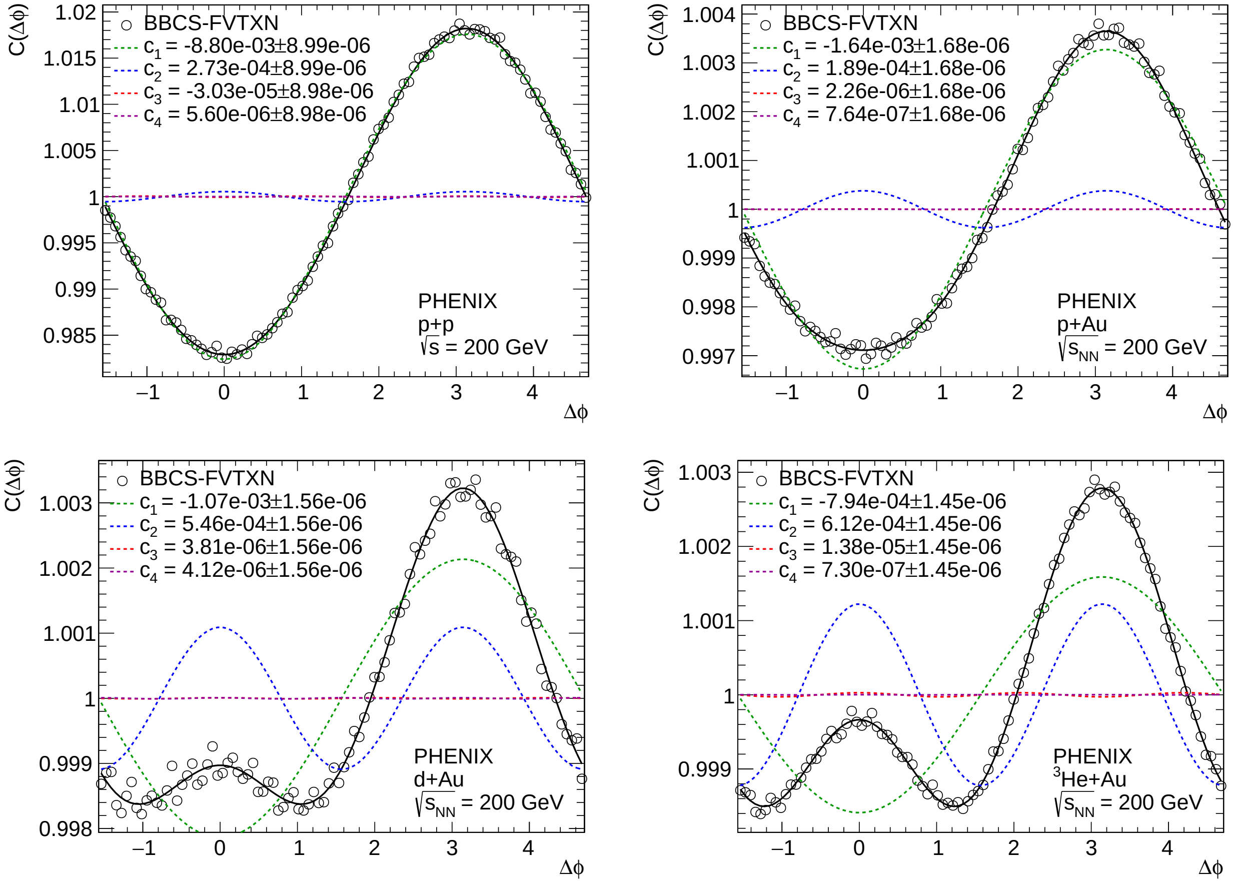


FIG. 14. BBCS-FVTXN $\Delta\phi$ distribution in MB $p$+$p$ and 0%–5% central $p$+Au, $d$+Au, and $^{3}$He+Au. The measured correlation function is shown with open black circles and the fit is shown as a solid black line.

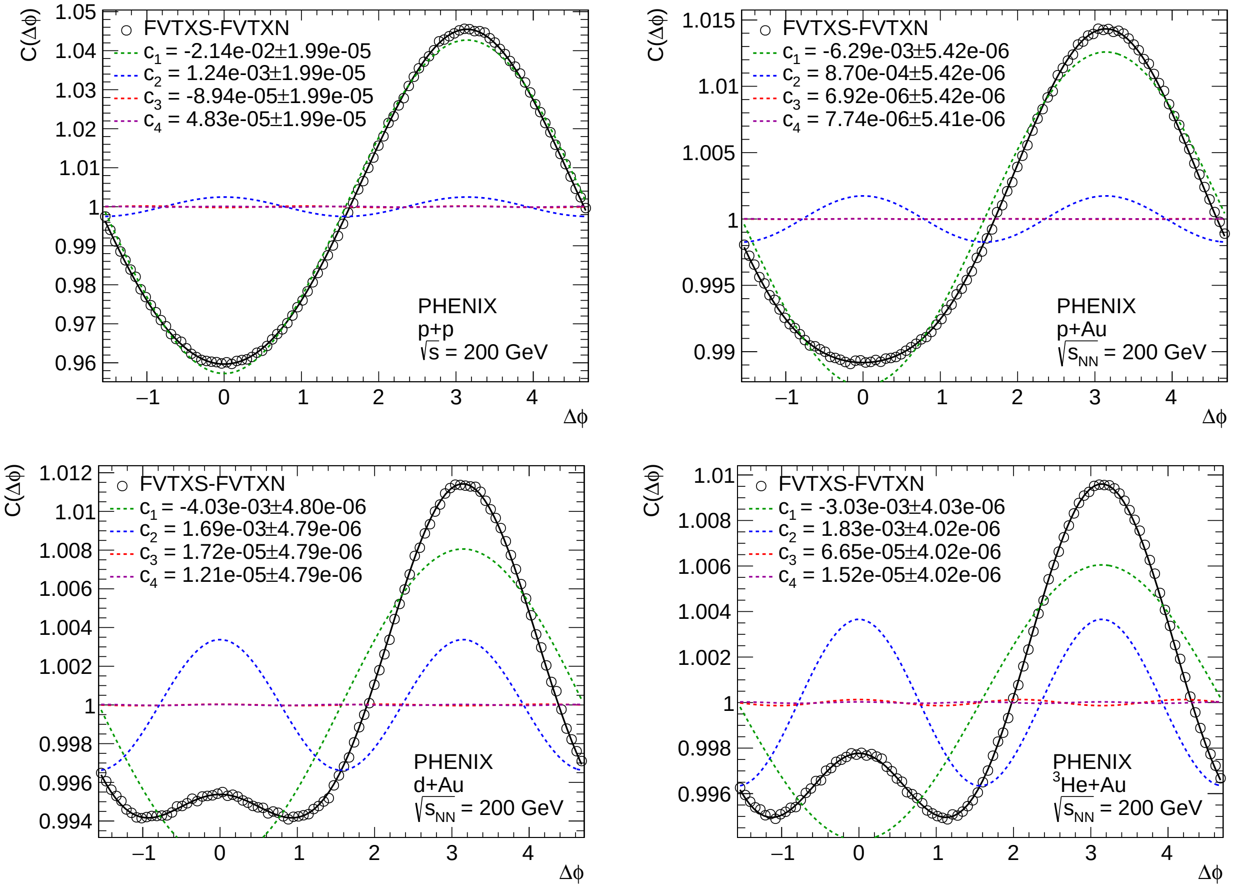


FIG. 15. FVTXS-FVTXN $\Delta\phi$ distribution in MB $p$+$p$ and 0%–5% central $p$+Au, $d$+Au, and $^3$He+Au. The measured correlation function is shown with open black circles and the fit is shown as a solid black line.

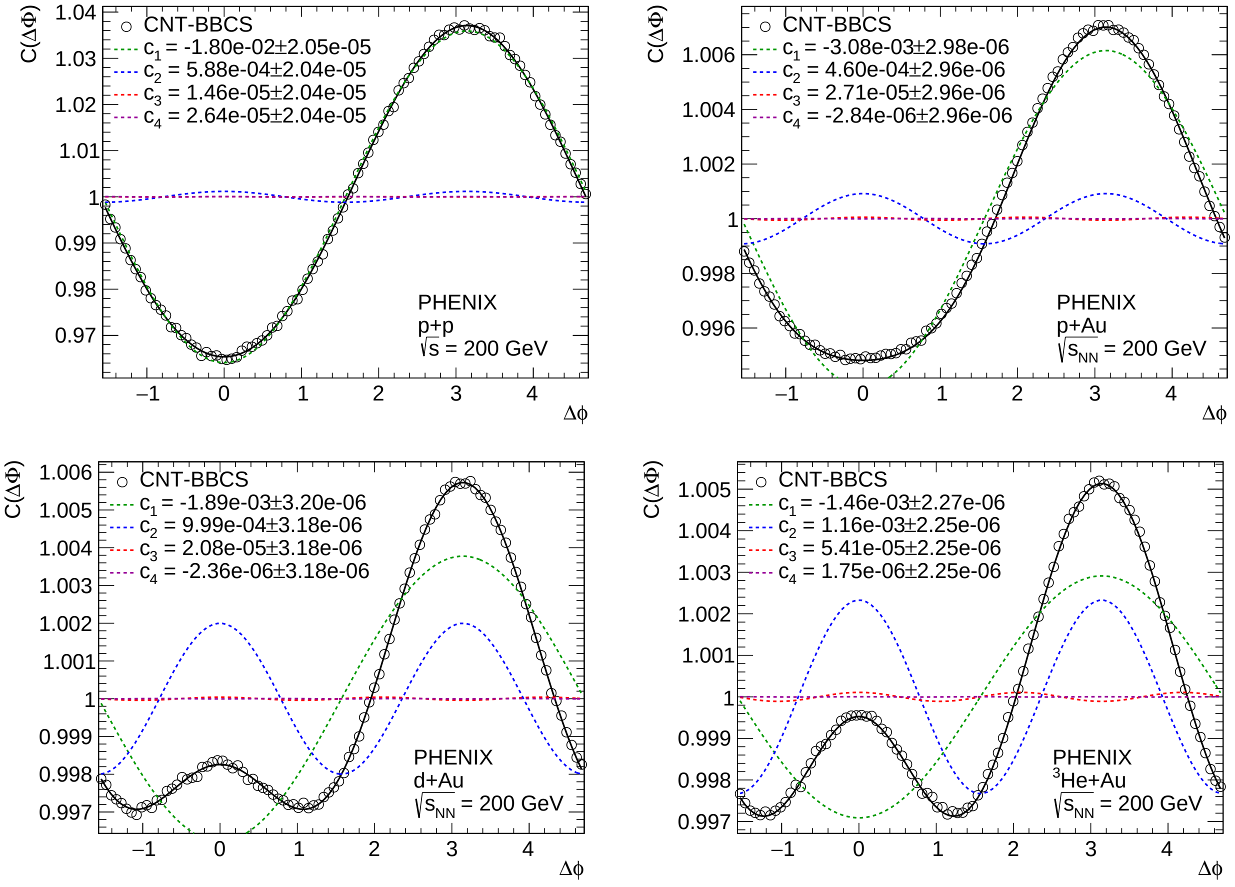


FIG. 16. CNT-BBCS $\Delta\phi$ distribution in MB $p$+$p$ and 0%–5% central $p$+Au, $d$+Au, and $^3$He+Au. The measured correlation function is shown with open black circles and the fit is shown as a solid black line.

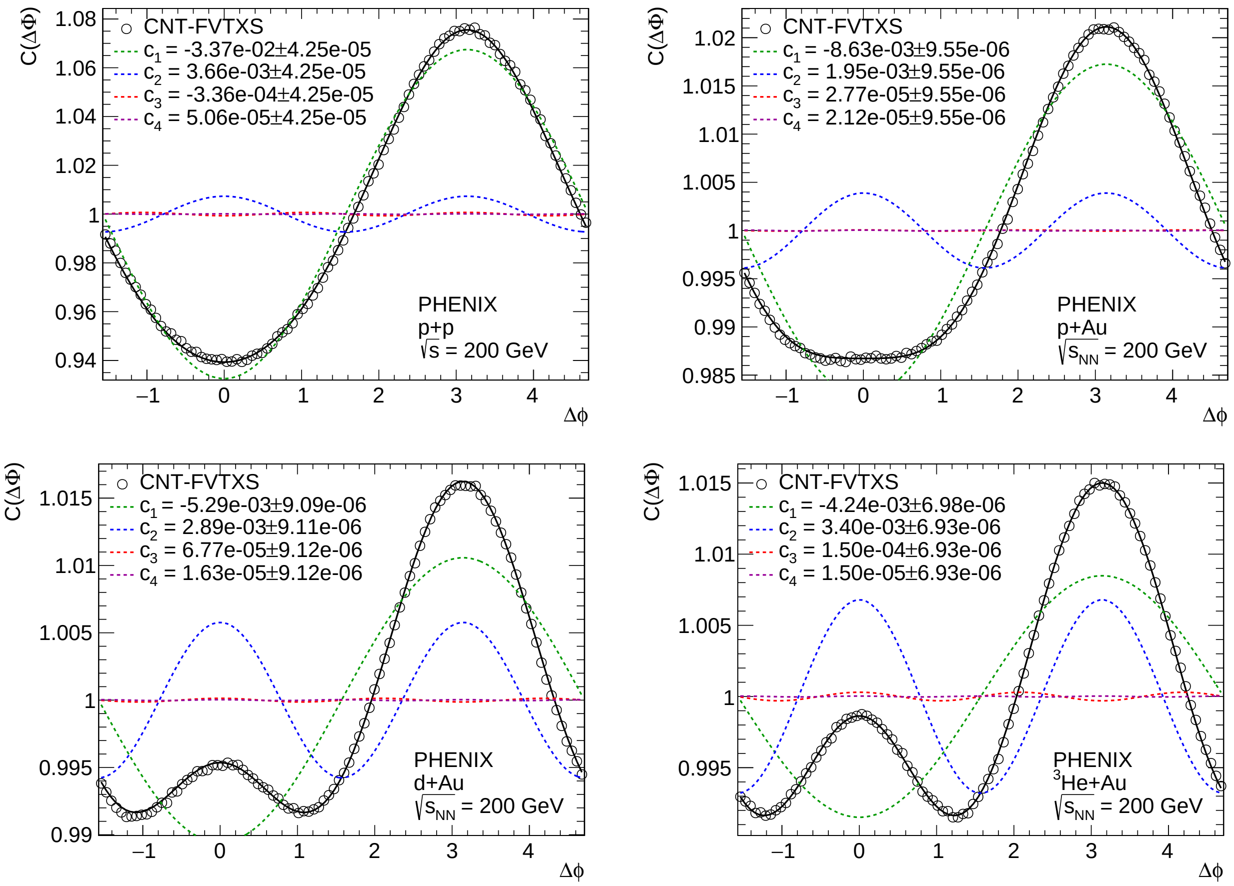


FIG. 17. CNT-FVTXS $\Delta\phi$ distribution in MB $p$+$p$ and 0%–5% central $p$+Au, $d$+Au, and $^3$He+Au. The measured correlation function is shown with open black circles and the fit is shown as a solid black line.

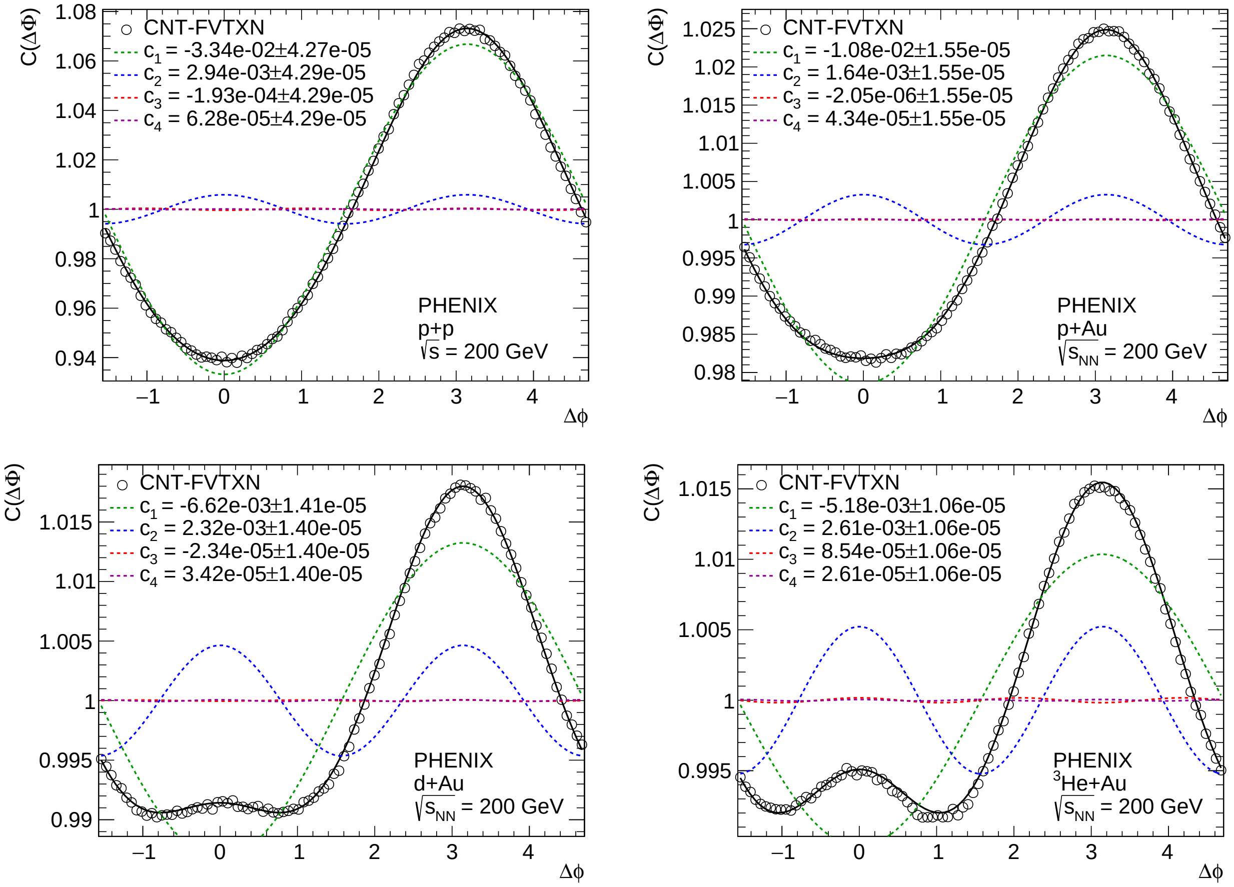


FIG. 18. CNT-FVTXN $\Delta\phi$ distribution in MB $p$+$p$ and 0%–5% central $p$+Au, $d$+Au, and $^3$He+Au. The measured correlation function is shown with open black circles and the fit is shown as a solid black line.

TABLE V. Table of $p_T$-integrated Fourier coefficients, $p$+$p$ collisions.

| | $c_1$ | $c_2$ | $c_3$ | $c_4$ |
|---|---|---|---|---|
| BBCS-FVTXS | -1.57e-02 ± 8.40e-06 | 1.38e-03 ± 8.39e-06 | 1.34e-06 ± 8.39e-06 | 2.55e-05 ± 8.39e-06 |
| BBCS-FVTXN | -8.80e-03 ± 8.99e-06 | 2.73e-04 ± 8.99e-06 | -3.03e-05 ± 8.98e-06 | 5.60e-06 ± 8.98e-06 |
| FVTXN-FVTXS | -2.14e-02 ± 1.99e-05 | 1.24e-03 ± 1.99e-05 | -8.94e-05 ± 1.99e-05 | 4.83e-05 ± 1.99e-05 |
| CNT-BBCS | -1.80e-02 ± 2.05e-05 | 5.88e-04 ± 2.04e-05 | 1.46e-05 ± 2.04e-05 | 2.64e-05 ± 2.04e-05 |
| CNT-FVTXS | -3.37e-02 ± 4.25e-05 | 3.66e-03 ± 4.25e-05 | -3.36e-04 ± 4.25e-05 | 5.06e-05 ± 4.25e-05 |
| CNT-FVTXN | -3.34e-02 ± 4.27e-05 | 2.94e-03 ± 4.29e-05 | -1.93e-04 ± 4.29e-05 | 6.28e-05 ± 4.29e-05 |

TABLE VI. Table of $p_T$-dependent Fourier coefficients, CNT-BBCS, $p$+$p$ collisions.

| $p_T$ (GeV/$c$) | $c_1$ | $c_2$ | $c_3$ | $c_4$ |
|---|---|---|---|---|
| 0.3 | -1.20e-02 ± 3.48e-05 | 2.90e-04 ± 3.47e-05 | 1.79e-05 ± 3.47e-05 | 9.97e-06 ± 3.47e-05 |
| 0.5 | -1.62e-02 ± 3.75e-05 | 4.00e-04 ± 3.73e-05 | 1.94e-05 ± 3.72e-05 | 5.43e-05 ± 3.73e-05 |
| 0.7 | -2.10e-02 ± 5.10e-05 | 6.58e-04 ± 5.05e-05 | -4.13e-05 ± 5.05e-05 | 7.24e-05 ± 5.06e-05 |
| 0.9 | -2.53e-02 ± 7.08e-05 | 1.06e-03 ± 7.02e-05 | -9.07e-05 ± 7.02e-05 | 4.89e-05 ± 7.02e-05 |
| 1.1 | -2.86e-02 ± 9.68e-05 | 1.39e-03 ± 9.59e-05 | -9.37e-05 ± 9.60e-05 | -6.00e-05 ± 9.59e-05 |
| 1.3 | -3.15e-02 ± 1.30e-04 | 1.94e-03 ± 1.29e-04 | -6.50e-04 ± 1.29e-04 | -5.03e-05 ± 1.28e-04 |
| 1.5 | -3.33e-02 ± 1.72e-04 | 1.79e-03 ± 1.70e-04 | -3.68e-04 ± 1.70e-04 | 4.28e-04 ± 1.70e-04 |
| 1.7 | -3.57e-02 ± 2.23e-04 | 2.14e-03 ± 2.21e-04 | -3.77e-04 ± 2.22e-04 | 2.19e-04 ± 2.21e-04 |
| 1.9 | -3.71e-02 ± 2.88e-04 | 2.52e-03 ± 2.85e-04 | -1.25e-04 ± 2.85e-04 | -5.00e-04 ± 2.84e-04 |
| 2.1 | -3.83e-02 ± 3.66e-04 | 3.44e-03 ± 3.62e-04 | 3.46e-04 ± 3.63e-04 | -4.12e-04 ± 3.61e-04 |
| 2.3 | -4.06e-02 ± 4.61e-04 | 3.96e-03 ± 4.56e-04 | -2.87e-04 ± 4.58e-04 | -1.29e-04 ± 4.56e-04 |
| 2.5 | -4.09e-02 ± 5.73e-04 | 2.52e-03 ± 5.67e-04 | 4.41e-04 ± 5.68e-04 | -2.46e-04 ± 5.66e-04 |
| 2.7 | -4.26e-02 ± 7.04e-04 | 2.58e-03 ± 6.97e-04 | -3.55e-04 ± 6.99e-04 | -9.45e-04 ± 6.96e-04 |
| 2.9 | -4.17e-02 ± 8.54e-04 | 4.39e-03 ± 8.45e-04 | -1.30e-03 ± 8.48e-04 | -9.99e-04 ± 8.44e-04 |

TABLE VII. Table of $p_T$-dependent Fourier coefficients, CNT-FVTXS, $p$+$p$ collisions.

| $p_T$ (GeV/$c$) | $c_1$ | $c_2$ | $c_3$ | $c_4$ |
|---|---|---|---|---|
| 0.3 | -2.10e-02 ± 7.32e-05 | 1.23e-03 ± 7.31e-05 | 9.42e-05 ± 7.31e-05 | 9.03e-05 ± 7.31e-05 |
| 0.5 | -2.94e-02 ± 7.84e-05 | 2.84e-03 ± 7.84e-05 | -1.53e-04 ± 7.84e-05 | 6.22e-05 ± 7.84e-05 |
| 0.7 | -3.86e-02 ± 1.05e-04 | 4.23e-03 ± 1.05e-04 | -5.11e-04 ± 1.05e-04 | -1.16e-04 ± 1.05e-04 |
| 0.9 | -4.74e-02 ± 1.44e-04 | 5.97e-03 ± 1.44e-04 | -7.94e-04 ± 1.44e-04 | 8.98e-05 ± 1.44e-04 |
| 1.1 | -5.47e-02 ± 1.94e-04 | 7.61e-03 ± 1.94e-04 | -1.09e-03 ± 1.94e-04 | 2.67e-04 ± 1.94e-04 |
| 1.3 | -6.08e-02 ± 2.58e-04 | 9.16e-03 ± 2.58e-04 | -8.06e-04 ± 2.58e-04 | -9.78e-05 ± 2.57e-04 |
| 1.5 | -6.80e-02 ± 3.38e-04 | 1.10e-02 ± 3.38e-04 | -1.65e-03 ± 3.38e-04 | 7.04e-04 ± 3.37e-04 |
| 1.7 | -7.32e-02 ± 4.37e-04 | 1.26e-02 ± 4.37e-04 | -2.74e-03 ± 4.38e-04 | 1.81e-04 ± 4.36e-04 |
| 1.9 | -7.86e-02 ± 5.60e-04 | 1.45e-02 ± 5.61e-04 | -2.39e-03 ± 5.61e-04 | 9.62e-04 ± 5.58e-04 |
| 2.1 | -8.39e-02 ± 7.08e-04 | 1.53e-02 ± 7.10e-04 | -3.44e-03 ± 7.10e-04 | 1.44e-03 ± 7.06e-04 |
| 2.3 | -8.97e-02 ± 8.89e-04 | 1.69e-02 ± 8.91e-04 | -3.81e-03 ± 8.91e-04 | 3.00e-04 ± 8.85e-04 |
| 2.5 | -9.27e-02 ± 1.10e-03 | 1.96e-02 ± 1.11e-03 | -4.71e-03 ± 1.10e-03 | 1.76e-03 ± 1.10e-03 |
| 2.7 | -9.70e-02 ± 1.35e-03 | 2.05e-02 ± 1.36e-03 | -4.24e-03 ± 1.35e-03 | 3.29e-03 ± 1.34e-03 |
| 2.9 | -1.03e-01 ± 1.64e-03 | 2.47e-02 ± 1.64e-03 | -7.01e-03 ± 1.64e-03 | -1.27e-03 ± 1.63e-03 |

TABLE VIII. Table of $p_T$-dependent Fourier coefficients, CNT-FVTXN, $p$+$p$ collisions.

| $p_T$ (GeV/$c$) | $c_1$ | $c_2$ | $c_3$ | $c_4$ |
|---|---|---|---|---|
| 0.3 | -2.08e-02 ± 7.37e-05 | 1.37e-03 ± 7.38e-05 | 5.82e-05 ± 7.37e-05 | 1.87e-04 ± 7.37e-05 |
| 0.5 | -2.90e-02 ± 7.87e-05 | 1.96e-03 ± 7.91e-05 | 4.56e-05 ± 7.90e-05 | -3.32e-05 ± 7.91e-05 |
| 0.7 | -3.82e-02 ± 1.05e-04 | 3.11e-03 ± 1.06e-04 | -8.13e-05 ± 1.06e-04 | -3.61e-05 ± 1.06e-04 |
| 0.9 | -4.69e-02 ± 1.44e-04 | 4.39e-03 ± 1.45e-04 | -4.56e-04 ± 1.45e-04 | -1.12e-05 ± 1.45e-04 |
| 1.1 | -5.44e-02 ± 1.95e-04 | 6.24e-03 ± 1.96e-04 | -6.33e-04 ± 1.96e-04 | 2.63e-04 ± 1.96e-04 |
| 1.3 | -6.05e-02 ± 2.59e-04 | 7.48e-03 ± 2.60e-04 | -1.21e-03 ± 2.60e-04 | 2.57e-04 ± 2.59e-04 |
| 1.5 | -6.69e-02 ± 3.39e-04 | 9.38e-03 ± 3.41e-04 | -1.05e-03 ± 3.41e-04 | 2.79e-05 ± 3.40e-04 |
| 1.7 | -7.36e-02 ± 4.39e-04 | 1.04e-02 ± 4.41e-04 | -2.23e-03 ± 4.42e-04 | 8.23e-04 ± 4.40e-04 |
| 1.9 | -7.81e-02 ± 5.62e-04 | 1.17e-02 ± 5.65e-04 | -1.85e-03 ± 5.65e-04 | 4.87e-04 ± 5.63e-04 |
| 2.1 | -8.37e-02 ± 7.10e-04 | 1.33e-02 ± 7.15e-04 | -2.52e-03 ± 7.15e-04 | 6.25e-04 ± 7.12e-04 |
| 2.3 | -8.83e-02 ± 8.94e-04 | 1.65e-02 ± 8.98e-04 | -3.61e-03 ± 8.98e-04 | -4.65e-05 ± 8.93e-04 |
| 2.5 | -9.31e-02 ± 1.11e-03 | 1.71e-02 ± 1.12e-03 | -1.54e-03 ± 1.12e-03 | 1.70e-03 ± 1.11e-03 |
| 2.7 | -9.69e-02 ± 1.36e-03 | 1.58e-02 ± 1.37e-03 | -2.59e-03 ± 1.37e-03 | 1.93e-03 ± 1.36e-03 |
| 2.9 | -1.04e-01 ± 1.64e-03 | 1.90e-02 ± 1.65e-03 | -6.63e-03 ± 1.65e-03 | -3.10e-03 ± 1.64e-03 |

TABLE IX. Table of $p_T$-integrated Fourier coefficients, $p$+Au collisions.

| | $c_1$ | $c_2$ | $c_3$ | $c_4$ |
|---|---|---|---|---|
| BBCS-FVTXS | -2.43e-03 ± 1.05e-06 | 5.10e-04 ± 1.05e-06 | 3.91e-05 ± 1.05e-06 | 5.00e-06 ± 1.05e-06 |
| BBCS-FVTXN | -1.64e-03 ± 1.68e-06 | 1.89e-04 ± 1.68e-06 | 2.26e-06 ± 1.68e-06 | 7.64e-07 ± 1.68e-06 |
| FVTXN-FVTXS | -6.29e-03 ± 5.42e-06 | 8.70e-04 ± 5.42e-06 | 6.92e-06 ± 5.42e-06 | 7.74e-06 ± 5.41e-06 |
| CNT-BBCS | -3.08e-03 ± 2.98e-06 | 4.60e-04 ± 2.96e-06 | 2.71e-05 ± 2.96e-06 | -2.84e-06 ± 2.96e-06 |
| CNT-FVTXS | -8.63e-03 ± 9.55e-06 | 1.95e-03 ± 9.55e-06 | 2.77e-05 ± 9.55e-06 | 2.12e-05 ± 9.55e-06 |
| CNT-FVTXN | -1.08e-02 ± 1.55e-05 | 1.64e-03 ± 1.55e-05 | -2.05e-06 ± 1.55e-05 | 4.34e-05 ± 1.55e-05 |

TABLE X. Table of $p_T$-dependent Fourier coefficients, CNT-BBCS, $p$+Au collisions.

| $p_T$ (GeV/$c$) | $c_1$ | $c_2$ | $c_3$ | $c_4$ |
|---|---|---|---|---|
| 0.3 | -2.16e-03 ± 4.85e-06 | 2.20e-04 ± 4.85e-06 | 1.57e-05 ± 4.85e-06 | -1.84e-06 ± 4.86e-06 |
| 0.5 | -2.78e-03 ± 6.05e-06 | 3.74e-04 ± 6.00e-06 | 8.31e-06 ± 6.00e-06 | -2.05e-06 ± 6.01e-06 |
| 0.7 | -3.36e-03 ± 7.71e-06 | 5.29e-04 ± 7.64e-06 | 2.29e-05 ± 7.64e-06 | 1.00e-06 ± 7.64e-06 |
| 0.9 | -3.91e-03 ± 1.00e-05 | 6.58e-04 ± 9.94e-06 | 2.16e-05 ± 9.94e-06 | 1.71e-05 ± 9.94e-06 |
| 1.1 | -4.45e-03 ± 1.29e-05 | 8.06e-04 ± 1.28e-05 | 5.67e-06 ± 1.28e-05 | -4.48e-05 ± 1.28e-05 |
| 1.3 | -4.87e-03 ± 1.65e-05 | 9.35e-04 ± 1.63e-05 | 4.27e-05 ± 1.63e-05 | -1.22e-05 ± 1.63e-05 |
| 1.5 | -5.31e-03 ± 2.09e-05 | 1.08e-03 ± 2.07e-05 | 6.73e-05 ± 2.07e-05 | -2.81e-05 ± 2.06e-05 |
| 1.7 | -5.74e-03 ± 2.63e-05 | 1.16e-03 ± 2.60e-05 | -2.14e-05 ± 2.60e-05 | -4.34e-06 ± 2.60e-05 |
| 1.9 | -6.14e-03 ± 3.30e-05 | 1.22e-03 ± 3.27e-05 | 1.12e-04 ± 3.27e-05 | -2.19e-05 ± 3.26e-05 |
| 2.1 | -6.47e-03 ± 4.11e-05 | 1.18e-03 ± 4.07e-05 | 4.99e-05 ± 4.07e-05 | 1.16e-05 ± 4.06e-05 |
| 2.3 | -6.74e-03 ± 5.11e-05 | 1.34e-03 ± 5.06e-05 | -1.14e-04 ± 5.07e-05 | 1.01e-04 ± 5.05e-05 |
| 2.5 | -7.03e-03 ± 6.29e-05 | 1.38e-03 ± 6.23e-05 | 2.06e-04 ± 6.24e-05 | -1.74e-04 ± 6.22e-05 |
| 2.7 | -7.23e-03 ± 7.67e-05 | 1.40e-03 ± 7.60e-05 | -2.96e-05 ± 7.61e-05 | 1.93e-04 ± 7.58e-05 |
| 2.9 | -7.47e-03 ± 9.32e-05 | 1.33e-03 ± 9.23e-05 | 8.79e-05 ± 9.24e-05 | -1.83e-04 ± 9.21e-05 |

TABLE XI. Table of $p_T$-dependent Fourier coefficients, CNT-FVTXS, $p$+Au collisions.

| $p_T$ (GeV/$c$) | $c_1$ | $c_2$ | $c_3$ | $c_4$ |
|---|---|---|---|---|
| 0.3 | -5.60e-03 ± 1.57e-05 | 9.45e-04 ± 1.57e-05 | -2.89e-05 ± 1.57e-05 | 4.24e-05 ± 1.57e-05 |
| 0.5 | -7.49e-03 ± 1.94e-05 | 1.54e-03 ± 1.94e-05 | 2.61e-05 ± 1.94e-05 | 2.57e-06 ± 1.94e-05 |
| 0.7 | -9.42e-03 ± 2.46e-05 | 2.16e-03 ± 2.46e-05 | 8.17e-05 ± 2.46e-05 | 1.89e-05 ± 2.46e-05 |
| 0.9 | -1.13e-02 ± 3.19e-05 | 2.77e-03 ± 3.19e-05 | 1.11e-04 ± 3.19e-05 | -5.60e-05 ± 3.19e-05 |
| 1.1 | -1.29e-02 ± 4.10e-05 | 3.37e-03 ± 4.11e-05 | 1.46e-04 ± 4.10e-05 | -9.11e-06 ± 4.10e-05 |
| 1.3 | -1.46e-02 ± 5.21e-05 | 4.00e-03 ± 5.22e-05 | 2.40e-04 ± 5.21e-05 | -3.64e-05 ± 5.22e-05 |
| 1.5 | -1.61e-02 ± 6.60e-05 | 4.57e-03 ± 6.61e-05 | 2.78e-04 ± 6.60e-05 | 1.33e-04 ± 6.60e-05 |
| 1.7 | -1.75e-02 ± 8.31e-05 | 4.92e-03 ± 8.31e-05 | 1.78e-04 ± 8.30e-05 | -8.20e-05 ± 8.30e-05 |
| 1.9 | -1.92e-02 ± 1.04e-04 | 5.53e-03 ± 1.04e-04 | 8.03e-05 ± 1.04e-04 | 3.97e-05 ± 1.04e-04 |
| 2.1 | -2.06e-02 ± 1.30e-04 | 5.96e-03 ± 1.30e-04 | 6.81e-05 ± 1.30e-04 | 9.27e-05 ± 1.30e-04 |
| 2.3 | -2.17e-02 ± 1.61e-04 | 6.35e-03 ± 1.61e-04 | -4.71e-06 ± 1.61e-04 | 2.10e-04 ± 1.61e-04 |
| 2.5 | -2.30e-02 ± 1.99e-04 | 6.47e-03 ± 1.99e-04 | -1.76e-04 ± 1.98e-04 | 1.08e-04 ± 1.98e-04 |
| 2.7 | -2.38e-02 ± 2.42e-04 | 6.98e-03 ± 2.42e-04 | 2.49e-04 ± 2.42e-04 | 6.86e-06 ± 2.42e-04 |
| 2.9 | -2.51e-02 ± 2.94e-04 | 7.78e-03 ± 2.94e-04 | -3.13e-04 ± 2.94e-04 | 2.14e-04 ± 2.94e-04 |

TABLE XII. Table of $p_T$-dependent Fourier coefficients, CNT-FVTXN, $p$+Au collisions.

| $p_T$ (GeV/$c$) | $c_1$ | $c_2$ | $c_3$ | $c_4$ |
|---|---|---|---|---|
| 0.3 | -6.69e-03 ± 2.54e-05 | 9.01e-04 ± 2.54e-05 | -8.91e-06 ± 2.54e-05 | -3.57e-06 ± 2.54e-05 |
| 0.5 | -9.22e-03 ± 3.13e-05 | 1.29e-03 ± 3.14e-05 | 3.70e-05 ± 3.14e-05 | 3.88e-05 ± 3.14e-05 |
| 0.7 | -1.18e-02 ± 3.98e-05 | 1.69e-03 ± 3.98e-05 | -1.39e-05 ± 3.98e-05 | -1.94e-05 ± 3.98e-05 |
| 0.9 | -1.42e-02 ± 5.16e-05 | 2.29e-03 ± 5.17e-05 | -3.01e-06 ± 5.17e-05 | 5.71e-05 ± 5.16e-05 |
| 1.1 | -1.65e-02 ± 6.64e-05 | 2.87e-03 ± 6.65e-05 | 4.82e-05 ± 6.65e-05 | 1.52e-04 ± 6.65e-05 |
| 1.3 | -1.88e-02 ± 8.45e-05 | 3.27e-03 ± 8.46e-05 | -6.18e-05 ± 8.46e-05 | 1.17e-04 ± 8.46e-05 |
| 1.5 | -2.13e-02 ± 1.07e-04 | 3.79e-03 ± 1.07e-04 | -5.53e-05 ± 1.07e-04 | 2.54e-04 ± 1.07e-04 |
| 1.7 | -2.34e-02 ± 1.35e-04 | 4.37e-03 ± 1.35e-04 | -1.22e-04 ± 1.35e-04 | 8.91e-05 ± 1.35e-04 |
| 1.9 | -2.55e-02 ± 1.69e-04 | 4.90e-03 ± 1.69e-04 | -1.57e-04 ± 1.69e-04 | -4.69e-05 ± 1.69e-04 |
| 2.1 | -2.72e-02 ± 2.11e-04 | 5.11e-03 ± 2.11e-04 | -6.82e-05 ± 2.11e-04 | 1.22e-04 ± 2.11e-04 |
| 2.3 | -2.91e-02 ± 2.62e-04 | 5.78e-03 ± 2.62e-04 | -2.73e-05 ± 2.62e-04 | 9.22e-05 ± 2.62e-04 |
| 2.5 | -3.09e-02 ± 3.23e-04 | 6.97e-03 ± 3.23e-04 | -7.55e-04 ± 3.22e-04 | 1.47e-04 ± 3.22e-04 |
| 2.7 | -3.28e-02 ± 3.94e-04 | 6.63e-03 ± 3.94e-04 | -3.99e-04 ± 3.94e-04 | -6.79e-05 ± 3.93e-04 |
| 2.9 | -3.43e-02 ± 4.78e-04 | 7.27e-03 ± 4.78e-04 | -1.07e-03 ± 4.78e-04 | -3.36e-04 ± 4.78e-04 |

TABLE XIII. Table of $p_T$-integrated Fourier coefficients, $d$+Au collisions.

| | $c_1$ | $c_2$ | $c_3$ | $c_4$ |
|---|---|---|---|---|
| BBCS-FVTXS | -1.49e-03 ± 1.02e-06 | 9.21e-04 ± 1.02e-06 | 3.25e-05 ± 1.02e-06 | -3.40e-06 ± 1.02e-06 |
| BBCS-FVTXN | -1.07e-03 ± 1.56e-06 | 5.46e-04 ± 1.56e-06 | 3.81e-06 ± 1.56e-06 | 4.12e-06 ± 1.56e-06 |
| FVTXN-FVTXS | -4.03e-03 ± 4.80e-06 | 1.69e-03 ± 4.79e-06 | 1.72e-05 ± 4.79e-06 | 1.21e-05 ± 4.79e-06 |
| CNT-BBCS | -1.89e-03 ± 3.20e-06 | 9.99e-04 ± 3.18e-06 | 2.08e-05 ± 3.18e-06 | -2.36e-06 ± 3.18e-06 |
| CNT-FVTXS | -5.29e-03 ± 9.09e-06 | 2.89e-03 ± 9.11e-06 | 6.77e-05 ± 9.12e-06 | 1.63e-05 ± 9.12e-06 |
| CNT-FVTXN | -6.62e-03 ± 1.41e-05 | 2.32e-03 ± 1.40e-05 | -2.34e-05 ± 1.40e-05 | 3.42e-05 ± 1.40e-05 |

TABLE XIV. Table of $p_T$-dependent Fourier coefficients, CNT-BBCS, $d$+Au collisions.

| $p_T$ (GeV/$c$) | $c_1$ | $c_2$ | $c_3$ | $c_4$ |
|---|---|---|---|---|
| 0.3 | -1.32e-03 ± 5.08e-06 | 4.97e-04 ± 5.08e-06 | 2.29e-06 ± 5.08e-06 | -5.53e-06 ± 5.08e-06 |
| 0.5 | -1.71e-03 ± 6.52e-06 | 8.42e-04 ± 6.47e-06 | 1.67e-06 ± 6.46e-06 | 1.78e-06 ± 6.49e-06 |
| 0.7 | -2.12e-03 ± 8.40e-06 | 1.19e-03 ± 8.33e-06 | 2.72e-05 ± 8.33e-06 | 2.44e-06 ± 8.35e-06 |
| 0.9 | -2.49e-03 ± 1.10e-05 | 1.52e-03 ± 1.09e-05 | 2.73e-05 ± 1.09e-05 | -1.07e-05 ± 1.09e-05 |
| 1.1 | -2.82e-03 ± 1.42e-05 | 1.77e-03 ± 1.41e-05 | 2.11e-05 ± 1.41e-05 | 2.86e-06 ± 1.41e-05 |
| 1.3 | -3.14e-03 ± 1.82e-05 | 1.98e-03 ± 1.80e-05 | 7.39e-05 ± 1.81e-05 | 1.11e-05 ± 1.80e-05 |
| 1.5 | -3.38e-03 ± 2.32e-05 | 2.11e-03 ± 2.30e-05 | 3.34e-05 ± 2.31e-05 | 3.38e-05 ± 2.30e-05 |
| 1.7 | -3.70e-03 ± 2.94e-05 | 2.26e-03 ± 2.92e-05 | 8.79e-05 ± 2.92e-05 | 1.80e-05 ± 2.91e-05 |
| 1.9 | -3.83e-03 ± 3.72e-05 | 2.34e-03 ± 3.68e-05 | 6.88e-05 ± 3.69e-05 | 9.75e-05 ± 3.67e-05 |
| 2.1 | -4.23e-03 ± 4.65e-05 | 2.46e-03 ± 4.60e-05 | 1.28e-04 ± 4.62e-05 | 9.48e-05 ± 4.59e-05 |
| 2.3 | -4.48e-03 ± 5.80e-05 | 2.46e-03 ± 5.74e-05 | 8.81e-06 ± 5.76e-05 | 2.75e-05 ± 5.73e-05 |
| 2.5 | -4.41e-03 ± 7.15e-05 | 2.33e-03 ± 7.08e-05 | 1.70e-04 ± 7.10e-05 | -2.27e-06 ± 7.06e-05 |
| 2.7 | -4.72e-03 ± 8.75e-05 | 2.52e-03 ± 8.66e-05 | 7.37e-05 ± 8.69e-05 | 2.89e-05 ± 8.64e-05 |
| 2.9 | -4.87e-03 ± 1.06e-04 | 2.53e-03 ± 1.05e-04 | 1.12e-06 ± 1.06e-04 | -1.17e-04 ± 1.05e-04 |

TABLE XV. Table of $p_T$-dependent Fourier coefficients, CNT-FVTXS, $d$+Au collisions.

| $p_T$ (GeV/$c$) | $c_1$ | $c_2$ | $c_3$ | $c_4$ |
|---|---|---|---|---|
| 0.3 | -3.39e-03 ± 1.47e-05 | 1.53e-03 ± 1.46e-05 | 5.06e-05 ± 1.46e-05 | 1.67e-05 ± 1.46e-05 |
| 0.5 | -4.57e-03 ± 1.85e-05 | 2.40e-03 ± 1.86e-05 | 5.01e-05 ± 1.86e-05 | 2.27e-05 ± 1.86e-05 |
| 0.7 | -5.87e-03 ± 2.36e-05 | 3.35e-03 ± 2.38e-05 | 5.49e-05 ± 2.38e-05 | 8.66e-06 ± 2.39e-05 |
| 0.9 | -7.10e-03 ± 3.07e-05 | 4.23e-03 ± 3.10e-05 | 4.27e-05 ± 3.10e-05 | 3.82e-05 ± 3.10e-05 |
| 1.1 | -8.23e-03 ± 3.97e-05 | 4.97e-03 ± 4.01e-05 | 1.30e-04 ± 4.02e-05 | 3.31e-05 ± 4.01e-05 |
| 1.3 | -9.31e-03 ± 5.08e-05 | 5.83e-03 ± 5.13e-05 | 1.52e-04 ± 5.14e-05 | -1.78e-06 ± 5.13e-05 |
| 1.5 | -1.05e-02 ± 6.48e-05 | 6.31e-03 ± 6.54e-05 | 1.37e-04 ± 6.55e-05 | 1.29e-04 ± 6.53e-05 |
| 1.7 | -1.14e-02 ± 8.20e-05 | 6.69e-03 ± 8.29e-05 | 2.20e-04 ± 8.29e-05 | 8.74e-05 ± 8.27e-05 |
| 1.9 | -1.25e-02 ± 1.04e-04 | 7.36e-03 ± 1.05e-04 | 6.11e-05 ± 1.05e-04 | 1.70e-04 ± 1.04e-04 |
| 2.1 | -1.32e-02 ± 1.29e-04 | 7.49e-03 ± 1.31e-04 | 5.70e-05 ± 1.31e-04 | -8.25e-06 ± 1.30e-04 |
| 2.3 | -1.43e-02 ± 1.61e-04 | 7.74e-03 ± 1.63e-04 | 2.97e-04 ± 1.63e-04 | -1.87e-04 ± 1.63e-04 |
| 2.5 | -1.49e-02 ± 1.99e-04 | 8.02e-03 ± 2.01e-04 | 7.40e-05 ± 2.01e-04 | 1.86e-06 ± 2.00e-04 |
| 2.7 | -1.58e-02 ± 2.44e-04 | 7.73e-03 ± 2.46e-04 | 4.28e-04 ± 2.46e-04 | 4.50e-04 ± 2.45e-04 |
| 2.9 | -1.58e-02 ± 2.96e-04 | 7.92e-03 ± 2.99e-04 | 1.59e-04 ± 3.00e-04 | 1.24e-05 ± 2.98e-04 |

TABLE XVI. Table of $p_T$-dependent Fourier coefficients, CNT-FVTXN, $d$+Au collisions.

| $p_T$ (GeV/$c$) | $c_1$ | $c_2$ | $c_3$ | $c_4$ |
|---|---|---|---|---|
| 0.3 | -4.09e-03 ± 2.25e-05 | 1.27e-03 ± 2.25e-05 | 7.77e-05 ± 2.25e-05 | 1.93e-05 ± 2.25e-05 |
| 0.5 | -5.70e-03 ± 2.86e-05 | 2.01e-03 ± 2.86e-05 | -1.79e-05 ± 2.85e-05 | 1.28e-05 ± 2.85e-05 |
| 0.7 | -7.37e-03 ± 3.67e-05 | 2.63e-03 ± 3.66e-05 | -7.68e-05 ± 3.66e-05 | 6.43e-05 ± 3.66e-05 |
| 0.9 | -9.18e-03 ± 4.77e-05 | 3.34e-03 ± 4.77e-05 | -1.29e-04 ± 4.77e-05 | -6.20e-06 ± 4.77e-05 |
| 1.1 | -1.05e-02 ± 6.18e-05 | 4.09e-03 ± 6.17e-05 | -1.73e-04 ± 6.18e-05 | 7.30e-05 ± 6.18e-05 |
| 1.3 | -1.21e-02 ± 7.91e-05 | 4.63e-03 ± 7.90e-05 | -1.35e-04 ± 7.92e-05 | 5.42e-05 ± 7.91e-05 |
| 1.5 | -1.35e-02 ± 1.01e-04 | 5.17e-03 ± 1.01e-04 | -1.67e-04 ± 1.01e-04 | -7.94e-05 ± 1.01e-04 |
| 1.7 | -1.49e-02 ± 1.28e-04 | 5.38e-03 ± 1.28e-04 | -5.54e-04 ± 1.28e-04 | 2.25e-04 ± 1.28e-04 |
| 1.9 | -1.61e-02 ± 1.61e-04 | 6.06e-03 ± 1.61e-04 | -4.70e-04 ± 1.61e-04 | -1.29e-04 ± 1.61e-04 |
| 2.1 | -1.75e-02 ± 2.02e-04 | 6.45e-03 ± 2.01e-04 | -3.52e-04 ± 2.02e-04 | -3.32e-05 ± 2.02e-04 |
| 2.3 | -1.93e-02 ± 2.52e-04 | 7.13e-03 ± 2.51e-04 | -5.01e-04 ± 2.52e-04 | 6.14e-04 ± 2.52e-04 |
| 2.5 | -2.02e-02 ± 3.10e-04 | 7.09e-03 ± 3.09e-04 | -5.61e-04 ± 3.10e-04 | 2.90e-04 ± 3.10e-04 |
| 2.7 | -2.09e-02 ± 3.80e-04 | 7.54e-03 ± 3.79e-04 | -5.48e-04 ± 3.80e-04 | -3.76e-04 ± 3.80e-04 |
| 2.9 | -2.18e-02 ± 4.62e-04 | 7.55e-03 ± 4.61e-04 | -8.89e-04 ± 4.62e-04 | 4.12e-04 ± 4.62e-04 |

TABLE XVII. Table of $p_T$-integrated Fourier coefficients, $^3$He+Au collisions.

| | $c_1$ | $c_2$ | $c_3$ | $c_4$ |
|---|---|---|---|---|
| BBCS-FVTXS | -1.04e-03 ± 9.45e-07 | 9.63e-04 ± 9.45e-07 | 4.73e-05 ± 9.45e-07 | 5.73e-06 ± 9.45e-07 |
| BBCS-FVTXN | -7.94e-04 ± 1.45e-06 | 6.12e-04 ± 1.45e-06 | 1.38e-05 ± 1.45e-06 | 7.30e-07 ± 1.45e-06 |
| FVTXN-FVTXS | -3.03e-03 ± 4.03e-06 | 1.83e-03 ± 4.02e-06 | 6.65e-05 ± 4.02e-06 | 1.52e-05 ± 4.02e-06 |
| CNT-BBCS | -1.46e-03 ± 2.27e-06 | 1.16e-03 ± 2.25e-06 | 5.41e-05 ± 2.25e-06 | 1.75e-06 ± 2.25e-06 |
| CNT-FVTXS | -4.24e-03 ± 6.98e-06 | 3.40e-03 ± 6.93e-06 | 1.50e-04 ± 6.93e-06 | 1.50e-05 ± 6.93e-06 |
| CNT-FVTXN | -5.18e-03 ± 1.06e-05 | 2.61e-03 ± 1.06e-05 | 8.54e-05 ± 1.06e-05 | 2.61e-05 ± 1.06e-05 |

TABLE XVIII. Table of $p_T$-dependent Fourier coefficients, CNT-BBCS, $^3$He+Au collisions.

| $p_T$ (GeV/$c$) | $c_1$ | $c_2$ | $c_3$ | $c_4$ |
|---|---|---|---|---|
| 0.3 | -9.99e-04 ± 4.11e-06 | 5.50e-04 ± 4.10e-06 | 1.73e-05 ± 4.10e-06 | -4.51e-06 ± 4.10e-06 |
| 0.5 | -1.25e-03 ± 4.43e-06 | 9.27e-04 ± 4.39e-06 | 3.17e-05 ± 4.39e-06 | 1.22e-05 ± 4.40e-06 |
| 0.7 | -1.50e-03 ± 5.59e-06 | 1.31e-03 ± 5.53e-06 | 5.54e-05 ± 5.52e-06 | -2.42e-06 ± 5.53e-06 |
| 0.9 | -1.76e-03 ± 7.11e-06 | 1.61e-03 ± 7.02e-06 | 7.60e-05 ± 7.02e-06 | 2.15e-05 ± 7.02e-06 |
| 1.1 | -2.03e-03 ± 9.07e-06 | 1.88e-03 ± 8.95e-06 | 1.04e-04 ± 8.95e-06 | 4.27e-06 ± 8.94e-06 |
| 1.3 | -2.23e-03 ± 1.15e-05 | 2.09e-03 ± 1.14e-05 | 8.70e-05 ± 1.14e-05 | 8.54e-06 ± 1.14e-05 |
| 1.5 | -2.49e-03 ± 1.46e-05 | 2.31e-03 ± 1.44e-05 | 1.41e-04 ± 1.44e-05 | 2.79e-05 ± 1.44e-05 |
| 1.7 | -2.65e-03 ± 1.84e-05 | 2.44e-03 ± 1.82e-05 | 1.72e-04 ± 1.82e-05 | -1.80e-05 ± 1.82e-05 |
| 1.9 | -2.90e-03 ± 2.32e-05 | 2.54e-03 ± 2.28e-05 | 1.41e-04 ± 2.29e-05 | 4.96e-05 ± 2.28e-05 |
| 2.1 | -2.98e-03 ± 2.89e-05 | 2.49e-03 ± 2.85e-05 | 1.30e-04 ± 2.85e-05 | 5.47e-05 ± 2.85e-05 |
| 2.3 | -3.20e-03 ± 3.59e-05 | 2.66e-03 ± 3.54e-05 | 1.93e-04 ± 3.54e-05 | -7.37e-05 ± 3.54e-05 |
| 2.5 | -3.48e-03 ± 4.43e-05 | 2.65e-03 ± 4.37e-05 | 1.03e-04 ± 4.37e-05 | 4.90e-05 ± 4.37e-05 |
| 2.7 | -3.25e-03 ± 5.41e-05 | 2.51e-03 ± 5.34e-05 | 9.37e-05 ± 5.34e-05 | 9.46e-05 ± 5.33e-05 |
| 2.9 | -3.70e-03 ± 6.59e-05 | 2.51e-03 ± 6.49e-05 | 2.23e-04 ± 6.50e-05 | 4.90e-05 ± 6.49e-05 |

TABLE XIX. Table of $p_T$-dependent Fourier coefficients, CNT-FVTXS, $^3$He+Au collisions.

| $p_T$ (GeV/$c$) | $c_1$ | $c_2$ | $c_3$ | $c_4$ |
|---|---|---|---|---|
| 0.3 | -2.64e-03 ± 1.27e-05 | 1.68e-03 ± 1.27e-05 | 4.31e-05 ± 1.27e-05 | 1.53e-05 ± 1.27e-05 |
| 0.5 | -3.47e-03 ± 1.37e-05 | 2.69e-03 ± 1.36e-05 | 7.34e-05 ± 1.36e-05 | -8.39e-06 ± 1.36e-05 |
| 0.7 | -4.41e-03 ± 1.72e-05 | 3.72e-03 ± 1.71e-05 | 1.47e-04 ± 1.70e-05 | 3.21e-05 ± 1.70e-05 |
| 0.9 | -5.25e-03 ± 2.18e-05 | 4.71e-03 ± 2.16e-05 | 2.27e-04 ± 2.16e-05 | 3.88e-05 ± 2.16e-05 |
| 1.1 | -6.12e-03 ± 2.78e-05 | 5.49e-03 ± 2.75e-05 | 3.41e-04 ± 2.75e-05 | 3.62e-05 ± 2.75e-05 |
| 1.3 | -6.90e-03 ± 3.54e-05 | 6.31e-03 ± 3.50e-05 | 3.56e-04 ± 3.50e-05 | 1.08e-04 ± 3.49e-05 |
| 1.5 | -7.78e-03 ± 4.48e-05 | 6.85e-03 ± 4.43e-05 | 3.79e-04 ± 4.42e-05 | 9.31e-05 ± 4.42e-05 |
| 1.7 | -8.48e-03 ± 5.65e-05 | 7.35e-03 ± 5.58e-05 | 5.15e-04 ± 5.58e-05 | 1.14e-04 ± 5.58e-05 |
| 1.9 | -9.20e-03 ± 7.10e-05 | 7.69e-03 ± 7.01e-05 | 3.31e-04 ± 7.01e-05 | 6.97e-05 ± 7.01e-05 |
| 2.1 | -9.81e-03 ± 8.85e-05 | 8.17e-03 ± 8.74e-05 | 4.03e-04 ± 8.74e-05 | 6.55e-05 ± 8.74e-05 |
| 2.3 | -1.07e-02 ± 1.10e-04 | 7.93e-03 ± 1.09e-04 | 4.13e-04 ± 1.09e-04 | 2.24e-04 ± 1.09e-04 |
| 2.5 | -1.14e-02 ± 1.36e-04 | 8.29e-03 ± 1.34e-04 | 3.80e-04 ± 1.34e-04 | 2.17e-04 ± 1.34e-04 |
| 2.7 | -1.22e-02 ± 1.66e-04 | 8.24e-03 ± 1.64e-04 | 4.22e-04 ± 1.64e-04 | 1.07e-05 ± 1.64e-04 |
| 2.9 | -1.25e-02 ± 2.02e-04 | 8.67e-03 ± 1.99e-04 | 3.27e-04 ± 1.99e-04 | 2.33e-04 ± 1.99e-04 |

TABLE XX. Table of $p_T$-dependent Fourier coefficients, CNT-FVTXN, $^3$He+Au collisions.

| $p_T$ (GeV/$c$) | $c_1$ | $c_2$ | $c_3$ | $c_4$ |
|---|---|---|---|---|
| 0.3 | -3.17e-03 ± 1.95e-05 | 1.35e-03 ± 1.94e-05 | 9.64e-05 ± 1.94e-05 | 4.01e-05 ± 1.94e-05 |
| 0.5 | -4.17e-03 ± 2.07e-05 | 2.06e-03 ± 2.08e-05 | 8.67e-05 ± 2.08e-05 | 2.11e-05 ± 2.08e-05 |
| 0.7 | -5.32e-03 ± 2.60e-05 | 2.78e-03 ± 2.62e-05 | 8.63e-05 ± 2.61e-05 | -4.98e-06 ± 2.62e-05 |
| 0.9 | -6.41e-03 ± 3.30e-05 | 3.56e-03 ± 3.32e-05 | 1.08e-04 ± 3.32e-05 | -3.97e-05 ± 3.32e-05 |
| 1.1 | -7.50e-03 ± 4.20e-05 | 4.19e-03 ± 4.23e-05 | 1.98e-04 ± 4.23e-05 | -2.78e-05 ± 4.22e-05 |
| 1.3 | -8.56e-03 ± 5.34e-05 | 4.80e-03 ± 5.37e-05 | 1.25e-04 ± 5.37e-05 | 9.25e-05 ± 5.36e-05 |
| 1.5 | -9.67e-03 ± 6.76e-05 | 5.14e-03 ± 6.79e-05 | 7.87e-05 ± 6.80e-05 | 1.48e-04 ± 6.79e-05 |
| 1.7 | -1.07e-02 ± 8.53e-05 | 5.89e-03 ± 8.57e-05 | 1.55e-04 ± 8.57e-05 | 6.67e-05 ± 8.56e-05 |
| 1.9 | -1.16e-02 ± 1.07e-04 | 6.16e-03 ± 1.08e-04 | 3.08e-04 ± 1.08e-04 | 8.98e-05 ± 1.08e-04 |
| 2.1 | -1.25e-02 ± 1.34e-04 | 6.41e-03 ± 1.34e-04 | 1.77e-04 ± 1.34e-04 | 1.63e-04 ± 1.34e-04 |
| 2.3 | -1.32e-02 ± 1.66e-04 | 6.31e-03 ± 1.67e-04 | 3.86e-05 ± 1.67e-04 | 3.22e-05 ± 1.67e-04 |
| 2.5 | -1.45e-02 ± 2.05e-04 | 7.06e-03 ± 2.06e-04 | -1.39e-04 ± 2.06e-04 | 3.55e-04 ± 2.06e-04 |
| 2.7 | -1.55e-02 ± 2.50e-04 | 6.82e-03 ± 2.51e-04 | 1.79e-04 ± 2.51e-04 | 3.02e-04 ± 2.51e-04 |
| 2.9 | -1.54e-02 ± 3.04e-04 | 6.73e-03 ± 3.06e-04 | 2.18e-04 ± 3.06e-04 | 3.57e-04 ± 3.06e-04 |
